# Supplementary material for: SCAN: Bootstrapping Contrastive Pre-training for Data Efficiency
Source: arXiv:2411.09126 source file (2024-11-14)
Supplement: Supplementary file 1 [file appendix.tex]

\section{SCAN Algorithm} \label{alg:prune}
We present a detailed algorithm of our proposed SCAN in Algorithm~\ref{alg:prune}. 
This algorithm is applicable to contrastive pre-training models including CLIP and MoCo.

\begin{algorithm}
\caption{Dataset Pruning of SCAN.} 

\KwIn{Full training data $\mathcal{D}$,
Number of training epochs $\tau_{stop}$,
Number of mutation epochs $\tau_{cos}$,
Pre-initialized losses $\mathcal{L}_{pre}$ and $\mathcal{L}_{cur}$,
Threshold value $T_{td}$ and an infinitesimal value $\epsilon$.
}
\KwOut{Pre-trained model $\mathcal{M}$}
\While{$\tau_{cur} < \tau_{stop}$}{
\tcp{Pre-Pruning Warm-Up}
\If{($\hat{\mathcal{L}}_{pre} - \hat{\mathcal{L}}_{cur}) / (\hat{\mathcal{L}}_{pre} + \epsilon) \geq T_{td}$}{  
\For{Batched sample $\mathcal{D}_t \in \mathcal{D}$}{ 
Forward and update $\mathcal{M}$ on $\mathcal{D}_t$; 
}

$\hat{\mathcal{L}}_{pre} \leftarrow \hat{\mathcal{L}}_{cur}$;

Get the updated current epoch loss $\hat{\mathcal{L}}_{cur}$;
}
\Else{
\tcp{Pruning Data Preparation}
\If{$\tau_{cur}$ mod $(\tau_{cos} + 1) = 0$}{ 
\For{Batched sample $\mathcal{D}_t \in \mathcal{D}$}{ 
Forward and update $\mathcal{M}$ on $\mathcal{D}_t$; 

Obtain \emph{redundant} set $\mathcal{D}_t^{red}$ and \emph{ill-matched} set $\mathcal{D}_t^{ill}$;

Obtain the overall pruning subset $\mathcal{D}_{t}^{'} = \mathcal{D}_{t}^{red} \, | \, \mathcal{D}_{t}^{ill}$;
}
Accumulate all the candidate pruning data $\mathcal{D}^{'}$;
}
\tcp{Dataset Mutation}
\Else{ 
Obtain the pruning ratio $\rho_{cur}$;

Randomly prune $\rho_{cur} |\mathcal{D}^{'}|$ samples from $\mathcal{D}^{'}$;

\For{Batched sample $\mathcal{D}_t \in \mathcal{D} \setminus \mathcal{D}^{'}_{\rho}$}{
Forward and update $\mathcal{M}$ on $\mathcal{D}_t$ 
}
}
}
$\tau_{cur} \leftarrow \tau_{cur} + 1$ 
}
\end{algorithm}

\begin{table*}
    \centering
    \caption{Batch sizes for pre-training and fine-tuning CLIP models.} \label{tab:batch-size}
    \scalebox{1.0}{
    \begin{tabular}{c|cc|cc|cc|c}
    \toprule
    PT      & RN50          & RN101             & ViT-S/32          & ViT-S/16          & ViT-B/32          & ViT-B/16          & Swin-Base     \\
    \midrule
    \cmark  & 256$\times$4  & 200$\times$4      & 800$\times$4      & 400$\times$4      & 480$\times$4      & 200$\times$4      & 100$\times$4  \\
    \midrule
    \xmark  & 384           & 225               & 1024              & 600               & 768               & 300               & 160           \\
    \bottomrule
    \end{tabular} 
    }
\end{table*}

\section{More Experimental Settings}
\subsection{Pre-Training Details} \label{sec:model-details}
Our primary objective in this study is to assess the efficacy of our proposed data-efficient method. 
Consequently, we did not conduct an extensive parameter search and instead utilized a universal setting across different models.

Due to limitations in computational resources, most of our pre-training experiments were conducted using four NVIDIA A5000 GPUs. 
Specifically, for CLIP models, we employed 32 epochs, a learning rate of 1e-3, and a weight decay of 0.1. 
Various batch sizes are detailed in Table~\ref{tab:batch-size}. 
For the downstream image classification task, we fine-tuned the pre-trained models on a single NVIDIA A100-40G GPU. 
Fine-tuning comprises 10 epochs with a learning rate of 1e-3 and a weight decay of 0.1.

Regarding the pre-training of MoCo, we utilized the original implementation\footnote{https://github.com/facebookresearch/moco-v3.}. 
We employed batch sizes of 600 and 370 for ViT-16/S and ViT-B/16, respectively.

\subsection{Compared Baselines} \label{sec:more-baselines}
We compared with the following four baselines in this work:
\begin{itemize}[leftmargin=2em]
\item \textbf{Random} prunes $\rho$ samples with randomness for each epoch. 
Notably, it falls under dynamic pruning methods as the pruned samples vary across epochs.
\item \textbf{SemDeDup}~\cite{semdedup} identifies the semantic duplicates based on embedding similarities. 
We used one public implementation\footnote{https://github.com/BAAI-DCAI/Dataset-Pruning/tree/main.}.
This method is applicable only to multi-modal models such as CLIP.
\item \textbf{D-Pruning}~\cite{d-pruning} estimate the parameter influence of a training example through the removal of it.
We utilized the official implementation\footnote{https://github.com/BAAI-DCAI/Dataset-Pruning/tree/main.} for CLIP models only.
We abandoned the use of MoCo due to its hard-to-configure running environment.
\item \textbf{Info-Batch}~\cite{info-batch} is a recent robust dataset pruning baseline.
It prunes a portion of less informative samples and then rescales the gradients of the remaining samples to approximate the original gradients.
We followed the original code\footnote{https://github.com/henryqin1997/InfoBatch.} to re-implement it for our experiments.
\end{itemize}

\section{More Experimental Results} \label{sec:more-exp}
We present additional fine-tuning results of CLIP in Table~\ref{tab:clip-3m-rest} and Table~\ref{tab:clip-12m-rest}. 
Furthermore, Table~\ref{tab:clip-linear} shows the results of linear probing for CLIP. 
It is evident that our proposed SCAN method consistently achieves superior performance across various settings.

\begin{table*}[t!]
    \centering
    \caption{Performance comparison of CLIP models on the \textbf{CC3M+} pre-trained datasets.
    \grey{CLIP} utilizes \textbf{4.1M} pre-trained data samples, while the remaining models use \textbf{2.9M}.
    The best results (excluding the original \grey{CLIP} model) are highlighted in \textbf{bold}.} 
    % \vspace{-1em}
    \scalebox{0.93}{
    \begin{tabular}{l|l|cc|cc|ccc}
    \toprule
    \multirow{2}{*}{Architecture}   & \multirow{2}{*}{Method}   & \multicolumn{2}{c|}{IN Zero-Shot} & \multirow{2}{*}{CIFAR10}  & \multirow{2}{*}{CIFAR100} & \multirow{2}{*}{IN}    & \multirow{2}{*}{IN-V2} &\multirow{2}{*}{IN-R} \\
    \cmidrule(lr){3-4}
                                    &                           & Top-1     & Top-5                 &                           &                           &                           &               & \\
    \midrule
    \multirow{6}{*}{RN50}           & \grey{CLIP}               & \grey{17.06}  & \grey{36.21}  & \grey{95.32}  & \grey{80.01}  & \grey{73.81}  & \grey{61.89}  & \grey{36.09} \\
    \cmidrule(lr){2-9}
                                    & Random                    & 11.02         & 25.23         & 94.01         & 75.12         & 70.22         & 58.04         & 31.80   \\
                                    & SemDeDup~\cite{semdedup}  & 11.98         & 26.30         & 94.53         & 76.81         & 71.51         & 58.79         & 32.31     \\
                                    & D-Pruning~\cite{d-pruning}& 11.72         & 26.65         & 94.48         & 76.73         & 71.11         & 58.79         & 31.88     \\
                                    & Info-Batch~\cite{info-batch}& 16.44       & \bf{36.74}    & 95.30         & 79.40         & \bf{73.01}    & \bf{61.49}    & \bf{35.04}     \\
    \cmidrule(lr){2-9}
                                    & SCAN                      & \bf{16.91}    & 35.79         & \bf{95.30}    & \bf{80.24}    & 72.91         & 60.59         & 34.53         \\   
    \midrule
    \multirow{6}{*}{ViT-S/32}       & \grey{CLIP}               & \grey{13.70}  & \grey{29.33}  & \grey{90.59}  & \grey{71.74}  & \grey{55.60}  & \grey{42.81}  & \grey{23.91}\\
    \cmidrule(lr){2-9}
                                    & Random                    & 06.57         & 16.19         & 86.61         & 60.18         & 48.87         & 34.48         & 17.98     \\
                                    & SemDeDup~\cite{semdedup}  & 05.33         & 14.05         & 85.16         & 59.87         & 47.39         & 35.56         & 17.70     \\
                                    & D-Pruning~\cite{d-pruning}& 04.78         & 12.91         & 84.21         & 57.96         & 46.53         & 34.77         & 16.88     \\
                                    & Info-Batch~\cite{info-batch}& 10.89       & 26.91         & 90.02         & 69.99         & 50.53         & 39.61         & 19.69     \\
    \cmidrule(lr){2-9}
                                    & SCAN                      & \bf{14.88}    & \bf{31.47}    & \bf{90.12}    & \bf{70.33}    & \bf{54.13}    & \bf{41.29}    & \bf{22.70}     \\ 
    \midrule
    \multirow{6}{*}{ViT-S/16}       & \grey{CLIP}               & \grey{18.41}  & \grey{37.41}  & \grey{96.09}  & \grey{81.31}  & \grey{68.49}  & \grey{55.79}  & \grey{29.52}  \\
    \cmidrule(lr){2-9}
                                    & Random                    & 07.80         & 21.53         & 93.58         & 72.11         & 62.13         & 49.63         & 19.01     \\
                                    & SemDeDup~\cite{semdedup}  & 09.57         & 22.00         & 93.43         & 74.37         & 62.30         & 48.89         & 23.04     \\
                                    & D-Pruning~\cite{d-pruning}& 08.60         & 20.35         & 93.26         & 73.72         & 61.70         & 48.97         & 22.46     \\
                                    & Info-Batch~\cite{info-batch}& 16.19       & 35.06         & \bf{95.64}    & 80.03         & 67.57         & 53.52         & \bf{27.64}     \\ 
    \cmidrule(lr){2-9}
                                    & SCAN                      & \bf{17.31}    & \bf{35.51}    & 95.53         & \bf{80.27}    & \bf{66.86}    & \bf{53.59}    & 27.34     \\
    \midrule
    \multirow{6}{*}{ViT-B/32}       & \grey{CLIP}               & \grey{14.97}  & \grey{32.02}  & \grey{94.43}  & \grey{77.72}  & \grey{58.33}  & \grey{45.70}  & \grey{25.59}  \\
    \cmidrule(lr){2-9}
                                    & Random                    & 07.44         & 18.88         & 89.96         & 69.41         & 50.43         & 40.62         & 18.07     \\
                                    & SemDeDup~\cite{semdedup}  & 07.20         & 17.50         & 90.88         & 70.13         & 50.99         & 38.34         & 19.76     \\
                                    & D-Pruning~\cite{d-pruning}& 06.51         & 16.13         & 60.07         & 69.11         & 50.01         & 38.43         & 19.03     \\
                                    & Info-Batch~\cite{info-batch}& 12.44       & 30.98         & 93.57         & 75.44         & 55.99         & 43.30         & \bf{24.64}     \\
    \cmidrule(lr){2-9}
                                    & SCAN                      & \bf{16.48}    & \bf{33.60}    & \bf{93.77}    & \bf{77.63}    & \bf{56.64}    & \bf{44.25}    & 24.10     \\  
    \bottomrule
    \end{tabular}
    }
    \label{tab:clip-3m-rest}
    % \vspace{-1em}
\end{table*}

\begin{table*}[t!]
    \centering
    \caption{Performance comparison of CLIP models on the \textbf{CC12M+} pre-trained datasets.
    \grey{CLIP} utilizes \textbf{10.1M} pre-trained data samples, while the remaining models use \textbf{7.1M}.
    The best results (excluding the original \grey{CLIP} model) are highlighted in \textbf{bold}. } 
    % \vspace{-1em}
    \scalebox{0.93}{
    \begin{tabular}{l|l|cc|cc|ccc}
    \toprule
    \multirow{2}{*}{Architecture}   & \multirow{2}{*}{Method}   & \multicolumn{2}{c|}{IN Zero-Shot} & \multirow{2}{*}{CIFAR10}  & \multirow{2}{*}{CIFAR100} & \multirow{2}{*}{IN}    & \multirow{2}{*}{IN-V2} &\multirow{2}{*}{IN-R} \\
    \cmidrule(lr){3-4}
                                    &                           & Top-1     & Top-5                 &                           &                           &                           &               & \\
    \midrule
    \multirow{6}{*}{RN50}           & \grey{CLIP}               & \grey{20.95}  & \grey{44.41}  & \grey{95.68}  & \grey{80.75}  & \grey{74.93}  & \grey{62.81}  & \grey{38.36} \\
    \cmidrule(lr){2-9}
                                    & Random                    & 12.39         & 35.96         & 94.89         & 76.96         & 71.65         & 59.71         & 32.03         \\
                                    & SemDeDup~\cite{semdedup}  & 15.89         & 36.76         & 95.00         & 78.12         & 72.46         & 60.01         & 33.86         \\
                                    & D-Pruning~\cite{d-pruning}& 11.19         & 26.53         & 94.31         & 77.69         & 71.96         & 59.19         & 33.44     \\
                                    & Info-Batch~\cite{info-batch}& 20.63       & 45.10         & \bf{95.68}    & 79.88         & 73.53         & 61.23         & 36.67       \\
    \cmidrule(lr){2-9}
                                    & SCAN                      & \bf{23.03}    & \bf{47.83}    & 95.63         & \bf{81.03}    & \bf{74.28}    & \bf{62.20}    & \bf{38.14}         \\   
    \midrule
    \multirow{6}{*}{ViT-S/32}       & \grey{CLIP}               & \grey{26.48}  & \grey{51.32}  & \grey{93.23}  & \grey{76.32}  & \grey{61.53}  & \grey{48.60}  & \grey{30.57}      \\
    \cmidrule(lr){2-9}
                                    & Random                    & 08.79         & 16.93         & 87.79         & 63.04         & 50.12         & 38.09         & 21.11      \\
                                    & SemDeDup~\cite{semdedup}  & 05.04         & 13.49         & 86.43         & 61.67         & 49.46         & 37.37         & 19.29     \\
                                    & D-Pruning~\cite{d-pruning}& 04.54         & 12.43         & 85.86         & 61.81         & 48.39         & 36.57         & 18.62     \\
                                    & Info-Batch~\cite{info-batch}& 10.07       & 26.63         & 91.11         & 67.94         & 53.47         & 40.91         & 20.77     \\
    \cmidrule(lr){2-9}
                                    & SCAN                      & \bf{25.27}    & \bf{50.08}    & \bf{91.86}    & \bf{75.27}    & \bf{59.87}    & \bf{46.96}    & \bf{27.86}     \\ 
    \midrule
    \multirow{6}{*}{ViT-S/16}       & \grey{CLIP}               & \grey{27.09}  & \grey{53.57}  & \grey{96.62}  & \grey{84.05}  & \grey{71.40}  & \grey{58.40}  & \grey{34.24}      \\
    \cmidrule(lr){2-9}
                                    & Random                    & 16.58         & 35.43         & 95.00         & 79.90         & 67.78         & 54.12         & 26.23     \\
                                    & SemDeDup~\cite{semdedup}  & 10.56         & 26.52         & 94.46         & 76.65         & 65.32         & 51.37         & 25.52    \\
                                    & D-Pruning~\cite{d-pruning}& 09.37         & 22.16         & 93.42         & 75.52         & 63.53         & 50.79         & 24.43     \\
                                    & Info-Batch~\cite{info-batch}& 21.28       & 45.56         & 96.09         & 82.13         & 68.87         & 55.90         & 29.58       \\
    \cmidrule(lr){2-9}
                                    & SCAN                      & \bf{28.46}    & \bf{54.56}    & \bf{96.24}    & \bf{83.32}    & \bf{70.40}    & \bf{57.10}    & \bf{31.85}     \\  
    \bottomrule
    \end{tabular}
    }
    \label{tab:clip-12m-rest}
    % \vspace{-1em}
\end{table*}

\begin{table*}[t!]
    \centering
    \caption{Linear probing results of six CLIP models.
    For the CC3M+ pre-trained datasets, \grey{CLIP} utilizes \textbf{4.1M} pre-trained data samples, while the remaining models use \textbf{2.9M}.
    For the CC12M+ pre-trained datasets, \grey{CLIP} utilizes \textbf{10.1M} pre-trained data samples, while the remaining models use \textbf{7.1M}.
    The best results (excluding the original \grey{CLIP} model) are highlighted in \textbf{bold}. 
    A dash (-) indicates the collapse of pre-training, resulting in impaired evaluation of downstream tasks.} 
    % \vspace{-1em}
    \scalebox{0.82}{
    \begin{tabular}{l|l|cc|ccc|cc|ccc}
    \toprule
    \multirow{2}{*}{Arc}            & \multirow{2}{*}{Method}   & \multicolumn{5}{c|}{CC3M+}                    & \multicolumn{5}{c}{CC12M+}                 \\
                                                                \cmidrule(lr){3-7}                              \cmidrule(lr){8-12}
                                                                && CF-10    & CF-100    & IN    & IN-V2 & IN-R  & CF-10 & CF-100    & IN    & IN-V2 & IN-R  \\
    \midrule
    \multirow{6}{*}{\rotatebox{90}{RN50}}           
                                    & \grey{CLIP}               & \grey{95.58} & \grey{80.31} & \grey{73.96} & \grey{61.60} & \grey{35.59} & \grey{95.69} & \grey{81.88} & \grey{74.96} & \grey{62.85} & \grey{38.57} \\
    \cmidrule(lr){2-12}
                                    & Random                    & 93.89     & 75.45     & 70.25     & 58.05     & 31.78     & 94.00     & 76.43     & 70.99     & 58.78     & 32.09         \\
                                    & SemDeDup~\cite{semdedup}  & 94.92     & 77.16     & 71.62     & 58.99     & 32.44     & 94.88     & 78.00     & 72.22     & 59.70     & 33.16         \\
                                    & D-Pruning~\cite{d-pruning}& 94.50     & 76.78     & 71.00     & 57.98     & 31.70     & 94.30     & 77.70     & 71.77     & 59.01     & 33.20 \\
                                    & Info-Batch~\cite{info-batch}& 95.29   & 79.39     & 73.07     & 61.03     & \bf{34.66}& \bf{95.66}& 79.84     & 73.23     & 61.10     & 36.63 \\
    \cmidrule(lr){2-12}
                                    & SCAN                      & \bf{95.46}& \bf{80.35}& \bf{73.07}& \bf{61.25}& 34.59     & 95.62     & \bf{81.28}& \bf{74.27}& \bf{62.66}& \bf{37.30}        \\   
    \midrule
    \multirow{6}{*}{\rotatebox{90}{RN101}}          
                                    & \grey{CLIP}               & \grey{95.92} & \grey{82.04} & \grey{75.10} & \grey{63.61} & \grey{38.78} & \grey{96.03} & \grey{82.73} & \grey{75.78} & \grey{63.93} & \grey{40.09} \\
    \cmidrule(lr){2-12}
                                    & Random                    & 95.00     & 78.13     & 73.79     & 60.20     & 36.12     & 95.02     & 78.34     & 73.99     & 60.27     & 36.13         \\
                                    & SemDeDup~\cite{semdedup}  & 94.84     & 79.25     & 74.08     & 61.94     & 36.74     & 95.01     & 78.02     & 73.89     & 59.91     & 33.80 \\
                                    & D-Pruning~\cite{d-pruning}& 94.79     & 72.12     & 73.74     & 61.66     & 35.64     & 94.78     & 78.83     & 74.08     & 61.28     & 37.09 \\
                                    & Info-Batch~\cite{info-batch}& 95.08   & 80.76     & 74.13     & 62.89     & 37.57     & 95.82     & 81.56     & 75.02     & 63.21     & 39.21 \\
    \cmidrule(lr){2-12}
                                    & SCAN                      & \bf{95.67}& \bf{81.36}& \bf{74.42}& \bf{63.07}& \bf{37.86}& \bf{95.93}& \bf{82.12}& \bf{75.61}& \bf{63.87}& \bf{39.32}        \\
    \midrule
    \multirow{6}{*}{\rotatebox{90}{ViT-S/32}}       
                                    & \grey{CLIP}               & \grey{91.65} & \grey{72.23} & \grey{55.52} & \grey{43.00} & \grey{23.48} & \grey{93.29} & \grey{77.06} & \grey{61.73} & \grey{48.84} & \grey{30.40} \\
    \cmidrule(lr){2-12}
                                    & Random                    & 87.00     & 61.31     & 49.97     & 36.07     & 20.88     & 87.79     & 63.04     & 50.12     & 38.09     & 21.11         \\
                                    & SemDeDup~\cite{semdedup}  & 83.46     & 60.06     & 47.65     & 35.51     & 17.61     & 86.23     & 61.77     & 49.20     & 37.10     & 19.11     \\
                                    & D-Pruning~\cite{d-pruning}& 84.21     & 58.73     & 46.57     & 35.03     & 16.95     & 85.82     & 61.09     & 47.99     & 36.58     & 18.00 \\
                                    & Info-Batch~\cite{info-batch}& 89.30   & 70.02     & 50.51     & 39.58     & 19.78     & 91.02     & 68.90     & 53.49     & 40.69     & 20.71     \\
    \cmidrule(lr){2-12}
                                    & SCAN                      & \bf{89.37}& \bf{71.05}& \bf{54.24}& \bf{41.30}& \bf{22.65}& \bf{91.88}& \bf{74.86}& \bf{59.90}& \bf{46.90}& \bf{27.90}        \\
    \midrule
    \multirow{6}{*}{\rotatebox{90}{ViT-S/16}}      
                                    & \grey{CLIP}               & \grey{96.09} & \grey{81.39} & \grey{68.49} & \grey{55.19} & \grey{29.06} & \grey{96.66} & \grey{84.35} & \grey{71.53} & \grey{58.56} & \grey{33.85} \\
    \cmidrule(lr){2-12}
                                    & Random                    & 93.62     & 73.37     & 63.02     & 49.96     & 20.62     & 94.90     & 79.91     & 67.90     & 54.10     & 26.24       \\
                                    & SemDeDup~\cite{semdedup}  & 93.21     & 73.85     & 62.34     & 49.40     & 22.54     & 94.00     & 77.01     & 64.45     & 51.40     & 25.51   \\
                                    & D-Pruning~\cite{d-pruning}& 93.28     & 73.09     & 61.67     & 48.99     & 22.48     & 93.41     & 75.43     & 63.42     & 50.77     & 24.41 \\
                                    & Info-Batch~\cite{info-batch}& 95.26   & \bf{80.46}& \bf{67.76}& 53.49     & 27.11     & 96.03     & 82.11     & 68.78     & 55.78     & 29.59 \\
    \cmidrule(lr){2-12} 
                                    & SCAN                      & \bf{95.31}& 80.00     & 67.04     & \bf{53.75}& \bf{27.41}& \bf{96.37}& \bf{82.71}& \bf{70.32}& \bf{57.17}& \bf{31.89}     \\
    \midrule
    \multirow{6}{*}{\rotatebox{90}{ViT-B/32}}       
                                    & \grey{CLIP}               & \grey{94.36} & \grey{77.84} & \grey{58.43} & \grey{45.79} & \grey{25.50} & \grey{95.65} & \grey{81.62} & \grey{63.40} & \grey{50.33} & \grey{31.28} \\
    \cmidrule(lr){2-12}
                                    & Random                    & 90.05     & 69.26     & 50.23     & 40.54     & 18.03     & 90.13     & 69.98     & 51.99     & 41.01     & 20.08         \\
                                    & SemDeDup~\cite{semdedup}  & 90.44     & 69.86     & 50.89     & 38.15     & 19.89     & 90.77     & 70.00     & 51.19     & 39.80     & 20.91 \\
                                    & D-Pruning~\cite{d-pruning}& 90.06     & 69.08     & 50.04     & 37.87     & 19.11     & 90.07     & 69.65     & 51.23     & 37.99     & 20.43 \\
                                    & Info-Batch~\cite{info-batch}& 93.54   & 75.49     & \bf{56.98}& 44.03     & 24.08     & -         & -         & -         & -         & -         \\
    \cmidrule(lr){2-12}
                                    & SCAN                      & \bf{94.00}& \bf{76.91}& 56.72     & \bf{44.12}& \bf{24.21}& \bf{95.05}& \bf{81.21}& \bf{61.96}& \bf{48.42}& \bf{29.53}        \\
    \midrule
   \multirow{6}{*}{\rotatebox{90}{ViT-B/16}}       
                                    & \grey{CLIP}               & \grey{96.27} & \grey{82.74} & \grey{70.87} & \grey{57.77} & \grey{29.82} & \grey{96.77} & \grey{84.48} & \grey{72.37} & \grey{59.07} & \grey{33.24} \\
    \cmidrule(lr){2-12}
                                    & Random                    & 91.60     & 73.61     & 50.59     & 40.52     & 21.72     & 94.56     & 76.67     & 67.57     & 54.40     & 27.10     \\
                                    & SemDeDup~\cite{semdedup}  & 94.16     & 76.34     & 66.60     & 53.13     & 25.60     & 94.17     & 76.66     & 67.10     & 53.39     & 27.11 \\
                                    & D-Pruning~\cite{d-pruning}& 93.48     & 75.41     & 65.90     & 52.69     & 24.57     & 93.88     & 75.99     & 65.98     & 53.00     & 26.05 \\
                                    & Info-Batch~\cite{info-batch}& 96.10   & 81.06     & \bf{70.30}& 56.10     & 28.48     & 96.12     & 81.78     & 71.34     & 56.25     & 31.12 \\
    \cmidrule(lr){2-12}
                                    & SCAN                      & \bf{96.16}& \bf{81.10}& 69.55     & \bf{56.48}& \bf{28.76}& \bf{96.12}& \bf{83.97}& \bf{71.82}& \bf{58.31}& \bf{32.48}        \\
    \bottomrule
    \end{tabular}
    }
    \label{tab:clip-linear}
    % \vspace{-1em}
\end{table*}

\noindent\textbf{Experimental Results on CLIP-Benchmark.} We utilized the CLIP-Benchmark tool to assess the performance of both CLIP and our SCAN method across 19 additional datasets. 
For this evaluation, we employed models pre-trained on the CC12M+ datasets. 
The results, presented in Table~\ref{tab:clip-benchmark}, demonstrate that our SCAN method delivers performance competitive with the original CLIP.

\begin{table}[htbp]
\centering
\caption{Comparison of ViT-B/32 and ViT-B/16 using CLIP and SCAN on CLIP-Benchmark.} \label{tab:clip-benchmark}
\begin{tabular}{l|cc|cc}
\toprule
\multirow{2}{*}{Dataset}    & \multicolumn{2}{c|}{ViT-B/32}     & \multicolumn{2}{c}{ViT-B/16}  \\
                            \cmidrule(lr){2-3}                  \cmidrule(lr){4-5}
                            & CLIP      & SCAN                  & CLIP      & SCAN              \\
\midrule
FER2013          & 18.50   & 22.27   & 18.36   & 20.77   \\ 
ImageNet-O       & 30.70   & 30.55   & 33.05   & 31.20   \\ 
ImageNet-R       & 29.23   & 31.91   & 31.08   & 29.67   \\ 
ImageNetv2       & 20.19   & 21.80   & 21.39   & 20.90   \\ 
ObjectNet        & 15.13   & 13.93   & 14.84   & 15.03   \\ 
rendered-sst2    & 50.08   & 49.92   & 51.12   & 50.02   \\ 
STL-10           & 85.18   & 86.06   & 85.11   & 85.04   \\ 
SUN397           & 40.55   & 41.02   & 41.95   & 41.29   \\ 
VOC-2007         & 47.22   & 42.62   & 52.59   & 48.48   \\ 
Caltech-101      & 64.93   & 68.56   & 65.63   & 65.46   \\ 
Dmlab            & 20.02   & 11.81   & 17.77   & 16.19   \\ 
DTD              & 15.66   & 16.44   & 16.24   & 13.83   \\ 
EuroSat          & 21.92   & 29.81   & 34.20   & 29.67   \\ 
Flowers          & 18.63   & 24.70   & 20.80   & 20.13   \\ 
KITTI            & 32.63   & 32.77   & 35.49   & 35.59   \\ 
PCam             & 50.33   & 52.23   & 50.32   & 52.69   \\ 
Pet              & 31.28   & 43.06   & 36.41   & 35.84   \\ 
RESISC45         & 23.41   & 23.05   & 21.28   & 19.38   \\ 
SVHN             & 16.99   & 06.97   & 09.73   & 07.86   \\ 
\bottomrule
\end{tabular}
\end{table}

\noindent\textbf{Results \emph{w.r.t.} Pre-defined Thresholds.}
To assess the impact of varying thresholds, we evaluated two model architectures, RN50 and ViT-B/32, using threshold values from 0.1 to 0.7, with a step size of 0.2. 
The ImageNet zero-shot performance results are summarized in the table below. 
As indicated, the models perform optimally at threshold values of 0.3 or 0.5. For simplicity and consistency, we selected a threshold of 0.3 for subsequent model evaluations.

\begin{table}[htbp]
\centering
\caption{Performance comparison of RN50 and ViT-B/32 at different thresholds.} \label{tab:threshold}
\begin{tabular}{c|cc|cc}
\toprule
\multirow{2}{*}{Threshold}  & \multicolumn{2}{c|}{RN50}     & \multicolumn{2}{c}{ViT-B/32}      \\
                            \cmidrule(lr){2-3}              \cmidrule(lr){4-5}
                            & Top-1     & Top-5             & Top-1     & Top-5                 \\
\midrule
0.1               & 15.80                 & 35.21                 & 14.75                      & 31.58                      \\ 
0.3               & 16.91                 & 35.79                 & 16.48                      & 33.60                      \\ 
0.5               & 18.22                 & 37.79                 & 16.04                      & 33.19                      \\ 
0.7               & 18.20                 & 37.78                 & 16.48                      & 33.23                      \\
\bottomrule
\end{tabular}
\end{table}

\noindent \textbf{Different Pruning Ratios of MoCo.}
The performance variations with different pruning ratios ($\rho$) for the MoCo model are depicted in Fig.~\ref{fig:moco-ratio}. 
It is evident that as the pruning ratios increase, there is a general degradation in performance.

\noindent \textbf{More Visualization of Ill-matched Samples from CLIP.}
We further visualize some ill-matched samples as indicated by SCAN in Fig.~\ref{fig:viz-rest}.

\begin{figure*}[t!]
  \centering
  \includegraphics[width=0.95\linewidth]{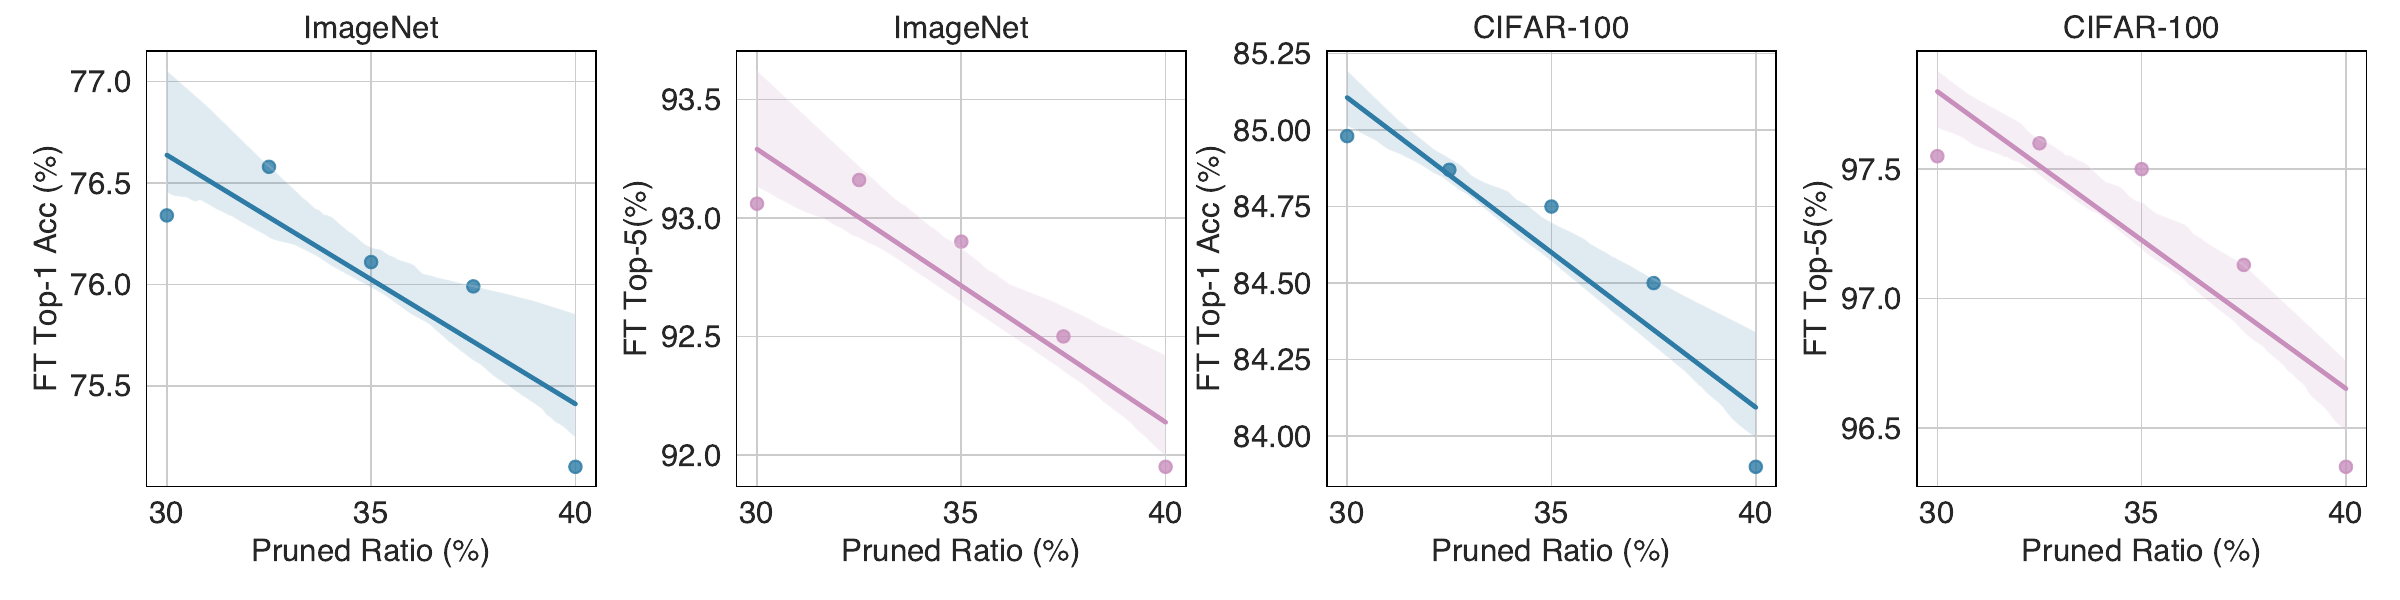}
  \caption{Downstream performance variation of ViT-S/16 MoCo model \emph{w.r.t.} different pruning ratios.}\label{fig:moco-ratio}
\end{figure*}

\begin{figure*}[t!]
  \centering
  \includegraphics[width=0.95\linewidth]{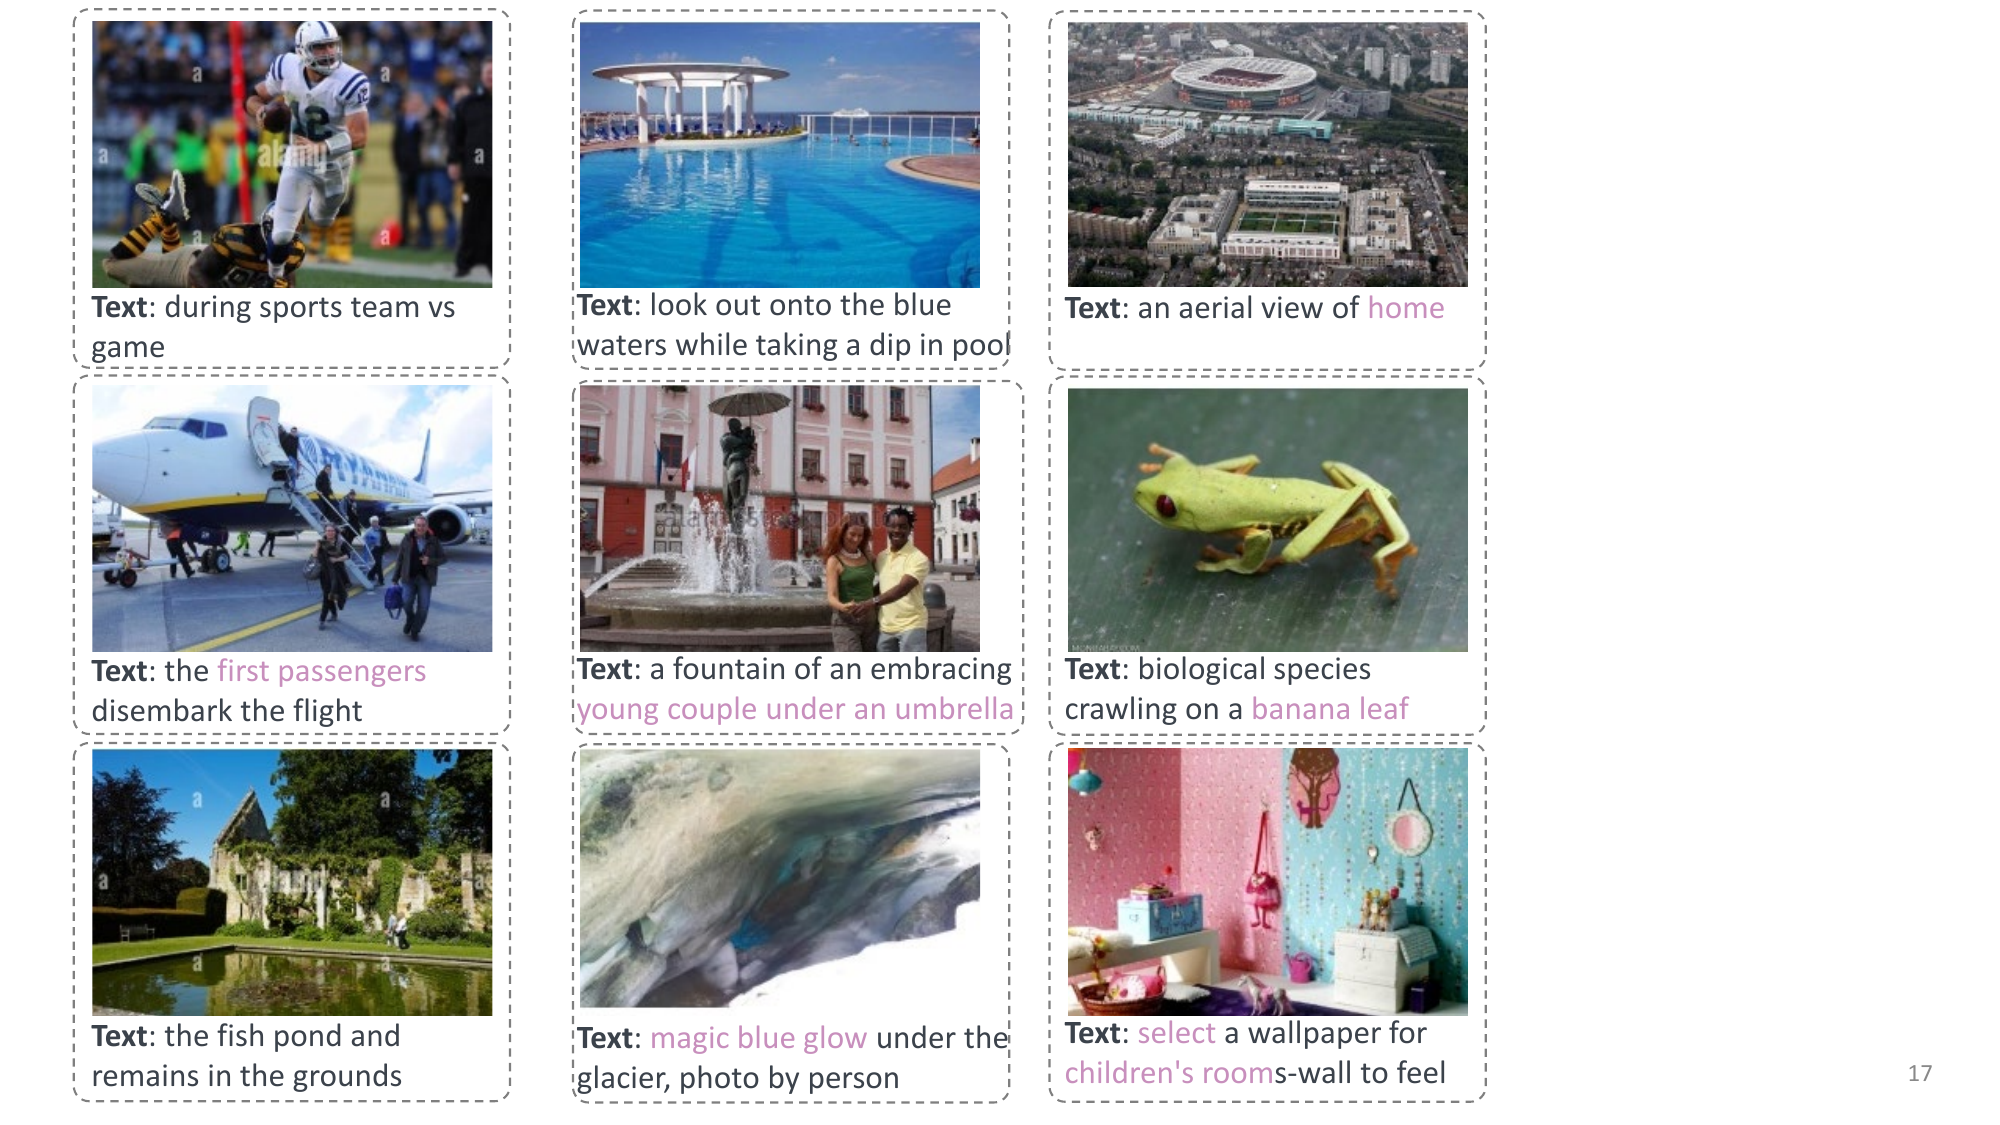}
  \caption{More \emph{ill-matched} samples obtained by our SCAN approach.}\label{fig:viz-rest}
\end{figure*}

% \newpage
